# Supplementary material for: PerfCodeGen: Improving Performance of LLM Generated Code with Execution Feedback
Source: arXiv:2412.03578 source file (2024-11-18)
Supplement: Supplementary file 1 [file ablation.tex]

\subsection{The Best@8 and Best@20 Results of Ablation Study}\label{a:ablation}

\begin{table}[t]
    \centering
    \begin{tabular}{c c c c c c c}
        \toprule
        \multirow{2}{*}{\textbf{Prompting Method}} & \multicolumn{2}{c}{\textbf{HumanEval}} & \multicolumn{2}{c}{\textbf{MBPP (test)}} & \multicolumn{2}{c}{\textbf{APPS (test)}} \\
        \cmidrule{2-7}
         & \textbf{Speedup} & \textbf{Opt\%} & \textbf{Speedup} & \textbf{Opt\%} & \textbf{Speedup} & \textbf{Opt\%}\\
        \midrule
        Base LLM (GPT-3.5) & 1.37 & 16.05 & 3.42 & 44.1 & 1.33 & 0.49 \\ \\
        \textbf{Single Round} & & & & & & \\
        Perf Improvement Prompt & \textbf{1.39} & 19.14 & 3.45 & 44.1 & 1.31 & 0.71 \\
        In-context learning & 1.38 & 19.14 & 3.20 & 44.98 & 1.31 & 0.74 \\
        Pre-defined Strategies & 1.27 & 16.67 & 2.86 & 32.75 & 1.31 & \textbf{0.77} \\ \\
        \textbf{Multi Round} & & & & & & \\
        Plan and Refine & 1.34 & 19.14 & 3.30 & 45.85 & 1.31 & 0.62 \\
        Analyze and Refine & 1.35 & 18.52 & 3.32 & 46.29 & 1.31 & 0.71 \\ \\
        \textbf{Multi Agent} & & & & & & \\
        Multi-Agent w/ Reviewer & 1.25 & 18.52 & 3.57 & 41.48 & 1.31 & 0.65 \\
        Multi-Agent w/ Team & 1.28 & 20.37 & 3.20 & 42.79 & 1.30 & 0.68 \\ \\
        \textbf{Exection Feedback} & & & & & & \\
        Direct Execution Feedback & 1.38 & 21.60 & 3.58 & 42.79 & 1.31 & 0.71 \\
        \tool & 1.34 & \textbf{22.22} & \textbf{4.19} & \textbf{47.16} & \textbf{1.32} & 0.58 \\
        \bottomrule \\
    \end{tabular}
    \caption{Results of different prompting schemes in the performance-refinement stage ($K$ of 1)}
    \label{tab:ablation_prompting_APPS}
\end{table}

\begin{table}[t]
    \centering
    \begin{tabular}{c | c c | c c}
        \toprule
        \multirow{2}*{\textbf{Prompting Method}} & \multicolumn{2}{c}{\textbf{GPT-3.5}} & \multicolumn{2}{c}{\textbf{Llama3 70B}} \\
        \cmidrule{2-5}
         &  \textbf{Speedup} & \textbf{Opt\%} & \textbf{Speedup} & \textbf{Opt\%}\\
        \midrule
        \multicolumn{5}{c}{\textbf{HumanEval}} \\
        \midrule
        Naive Prompting & 1.86 & 32.72 & 1.67 & 35.98  \\
        Few Shot Prompting (ICL) & 2.11 & 32.72 & 1.61 & 31.1 \\
        Pre-defined strategy & 2.17 & 28.4 & 1.60 & 30.49 \\ 
        Chain of Thought & 2.28 & 37.65 & 1.67 & \textbf{42.68} \\
        Time Complexity Optimization & \textbf{2.37} & 35.8 & 1.70 & 39.02  \\ 
        Multi-Agent w/ Reviewer & 2.27 & 36.42 & 1.68 & 39.02  \\ 
        Multi-Agent w/ Team & 2.24 & 38.27 & 1.67 & 42.07  \\ 
        Naive Execution Feedback & 2.27 & \textbf{40.74} & \textbf{1.71} & 39.63  \\ 
        \tool & 2.33 & 38.89 & \textbf{1.71} & 39.02  \\ 
        \midrule
        \multicolumn{5}{c}{\textbf{MBPP (test)}} \\ %\hline
        \midrule
         Naive Prompting & 3.94 & 66.81 & 2.43 & 32.88  \\
        Few Shot Prompting (ICL) & 3.93 & 65.94 & 2.48 & 34.68  \\
        Pre-defined strategy & 3.64 & 56.33 & 2.72 & 33.33  \\ 
        Chain of Thought & 3.32 & 70.31 & \textbf{3.33} & \textbf{39.19} \\
        Time Complexity Optimization & 3.58 & 67.25 & 3.05 & \textbf{39.19}  \\ 
        Multi-Agent w/ Reviewer & 4.10 & 67.25& 2.35 & 33.33  \\ 
        Multi-Agent w/ Team & 3.98 & \textbf{71.18} & 2.27 & 35.14  \\ 
        Naive Execution Feedback & 4.11 & 67.25 & 2.71 & 38.74  \\ 
        \tool &\textbf{ 4.13 }& \textbf{71.18} & 2.21 & 34.68 \\ 
        \midrule
        \multicolumn{5}{c}{\textbf{APPS (test)}} \\ %\hline
        \midrule
         Naive Prompting & 1.24 & 1.39 & 1.04 & 0.86 \\
        Few Shot Prompting (ICL) & 1.23 & 1.51 & 1.04 & 0.83  \\
        Pre-defined strategy & 1.23 & 1.45 & 1.04 & 0.77  \\ 
        Chain of Thought & 1.23 & 1.35 & 1.04 & \textbf{0.9}  \\
        Time Complexity Optimization & 1.24 & 1.35 & 1.04 & 0.86  \\ 
        Multi-Agent w/ Reviewer & 1.24 & 1.42 & 1.04 & 0.9 \\ 
        Multi-Agent w/ Team & \textbf{1.25} & 1.48 & 1.04 & 0.83  \\ 
        Naive Execution Feedback & 1.24 & \textbf{1.57} & 1.04 & 0.86  \\ 
        \tool & 1.24 & 1.48 & 1.04 & 0.86  \\ 
        \bottomrule
    \end{tabular}
    
    \caption{Best@8}
    \label{tab:ablation_best8}
\end{table}

\begin{table}[t]
    \centering
    \begin{tabular}{c | c c | c c}
        \toprule
        \multirow{2}*{\textbf{Prompting Method}} & \multicolumn{2}{c}{\textbf{GPT-3.5}} & \multicolumn{2}{c}{\textbf{Llama3 70B}} \\
        \cmidrule{2-5}
         &  \textbf{Speedup} & \textbf{Opt\%} & \textbf{Speedup} & \textbf{Opt\%}\\
        \midrule
        \multicolumn{5}{c}{\textbf{HumanEval}} \\
        \midrule
        Naive Prompting & 2.34 & 36.42 & 1.74 & 40.24  \\
        Few Shot Prompting (ICL) & 2.15 & 35.19 &1.68 & 35.98 \\
        Pre-defined strategy & 2.15 & 30.86 & 1.65 & 33.54 \\ 
        Chain of Thought & 2.28 & 43.21 & 1.79 & \textbf{46.95} \\
        Time Complexity Optimization & 2.34 & 41.98 & 1.79 & 46.34  \\ 
        Multi-Agent w/ Reviewer & 2.30 & 43.21 & 1.75 & 44.51  \\ 
        Multi-Agent w/ Team & 2.27 & 46.3 & 1.74 & 48.17  \\ 
        Naive Execution Feedback & 2.28 & \textbf{45.68} & \textbf{1.86} & 45.12  \\ 
        \tool & \textbf{2.33} & 43.21 & 1.84 & 45.73  \\ 
        \midrule
        \multicolumn{5}{c}{\textbf{MBPP (test)}} \\ %\hline
        \midrule
         Naive Prompting & 4.29 & 72.93 & 3.09 & 42.34  \\
        Few Shot Prompting (ICL) & 4.19 & 69.87 & 3.07 & 40.54  \\
        Pre-defined strategy & 3.94 & 61.14 & 3.13 & 38.74  \\ 
        Chain of Thought & 4.27 & 76.86 & \textbf{3.59} & \textbf{48.20} \\
        Time Complexity Optimization & 4.18 & 75.11 & 3.45 & 46.85  \\ 
        Multi-Agent w/ Reviewer & \textbf{4.40} & 74.24 & 3.21 & 45.05  \\ 
        Multi-Agent w/ Team & \textbf{4.40} & \textbf{77.29} & 2.76 & 43.69  \\ 
        Naive Execution Feedback & 4.31 & 74.67 & 3.23 & 45.50  \\ 
        \tool & 4.25 & 75.98 &2.88 & 44.59  \\ 
        \midrule
        \multicolumn{5}{c}{\textbf{APPS (test)}} \\ %\hline
        \midrule
         Naive Prompting & 1.23 & 1.91 & \textbf{1.07} & 1.36 \\
        Few Shot Prompting (ICL) & 1.23 & 2.06 & 1.06 & 1.14  \\
        Pre-defined strategy & 1.23 & 2.00 & 1.06 & 1.11  \\ 
        Chain of Thought & 1.23 & 1.94 & 1.06 & 1.23  \\
        Time Complexity Optimization & 1.23 & 2.06 & 1.06 & 1.27  \\ 
        Multi-Agent w/ Reviewer & 1.23 & 2.09 & \textbf{1.07} & 1.27 \\ 
        Multi-Agent w/ Team & 1.23 & 2.15 & \textbf{1.07} & 1.23  \\ 
        Naive Execution Feedback & 1.23 & \textbf{2.28} & \textbf{1.07} & 1.30  \\ 
        \tool & \textbf{1.24} & 2.06 & 1.06 & \textbf{1.39}  \\ 
        \bottomrule
    \end{tabular}
    
    \caption{Best@20}
    \label{tab:ablation_best20}
\end{table}
